# Supplementary material for: Designing a Multi-Objective Reward Function for Creating Teams of Robotic Bodyguards Using Deep Reinforcement Learning
Source: arXiv:1901.09837 source file (2019-01-28)
Supplement: Supplementary file 1 [file Appendix.tex]

\newpage
\section{Appendix}
\label{sec:Appendix}

\begin{table}[H]
\caption{Classification accuracies for naive Bayes and flexible
Bayes on various data sets.}
\label{sample-table}
\vskip 0.15in
\begin{center}
\begin{small}
\begin{sc}
\begin{tabular}{lcccr}
\toprule
Data set & Naive & Flexible & Better? \\
\midrule
Breast    & 95.9$\pm$ 0.2& 96.7$\pm$ 0.2& $\surd$ \\
Cleveland & 83.3$\pm$ 0.6& 80.0$\pm$ 0.6& $\times$\\
Glass2    & 61.9$\pm$ 1.4& 83.8$\pm$ 0.7& $\surd$ \\
Credit    & 74.8$\pm$ 0.5& 78.3$\pm$ 0.6&         \\
Horse     & 73.3$\pm$ 0.9& 69.7$\pm$ 1.0& $\times$\\
Meta      & 67.1$\pm$ 0.6& 76.5$\pm$ 0.5& $\surd$ \\
Pima      & 75.1$\pm$ 0.6& 73.9$\pm$ 0.5&         \\
Vehicle   & 44.9$\pm$ 0.6& 61.5$\pm$ 0.4& $\surd$ \\
\bottomrule
\end{tabular}
\end{sc}
\end{small}
\end{center}
\vskip -0.1in
\end{table}
\begin{table}[]
\centering
\caption{DDPG Binary Threat Function}
\label{tb:DDPG_binary_threat_function}
\begin{tabular}{llllll}
Two Agents Communication On & Two Agents Communication Off & Three Agents Communication On & Three Agents Communication Off & Four Agents Communication On & Four Agents Communication Off \\
1.673517574                 & 1.521234805                  & 1.479396322                   & 1.508775311                    & 1.385040947                  & 1.418334757                   \\
1.532865916                 & 1.8588788                    & 1.476488006                   & 1.549141317                    & 1.449169932                  & 1.690610886                   \\
1.857046448                 & 1.548972877                  & 1.555195425                   & 1.570449876                    & 1.427150221                  & 1.445620903                   \\
1.409117047                 & 1.429797988                  & 1.378090131                   & 1.613075246                    & 1.511915858                  & 1.416411687                   \\
1.479396322                 & 1.423218649                  & 1.3940496                     & 1.45646737                     & 1.307214166                  & 1.377957728
\end{tabular}
\end{table}

\begin{table}[]
\centering
\caption{DDPG Composite Reward Function}
\label{tab:DDPG-Composite-Reward}
\begin{tabular}{lll}
Two Agents  & Three Agents & Four Agents \\
1.269036039 & 1.340996147  & 1.481625867 \\
1.608443627 & 1.483757702  & 1.226568819 \\
1.503232505 & 1.383099255  & 1.166175475 \\
1.861512919 & 1.284498653  & 1.381713947 \\
1.510845221 & 1.409599464  & 1.254002966
\end{tabular}
\end{table}

\begin{table}[]
\centering
\caption{DDPG Composite Reward Function}
\label{tab:UnknownResults}
\begin{tabular}{llllll}
Two Agents Communication Off & Two Agents Communication On & Three Agents Communication Off & Three Agents Communication On & Four Agents Communication Off & Four Agents Communication On \\
1.604286284                  & 1.35171193                  & 1.352641585                    & 1.513132161                   & 1.494068638                   & 1.737719436                  \\
1.322924704                  & 1.436980808                 & 1.540043138                    & 1.615321559                   & 1.532354329                   & 1.356270044                  \\
1.474706047                  & 1.649564692                 & 1.554746269                    & 1.56317215                    & 1.257657372                   & 1.585083342                  \\
1.626695196                  & 1.446739362                 & 1.61698224                     & 1.607275284                   & 1.394123111                   & 1.716400649                  \\
1.453140131                  & 1.519955815                 & 1.519447882                    & 1.540522991                   & 1.466872532                   & 1.623664374
\end{tabular}
\end{table}

\begin{table}[]
\centering
\caption{My caption}
\label{tab:UnknownResults2}
\begin{tabular}{llllll}
Two Agents Communication Off & Two Agents Communication On & Three Agents Communication Off & Three Agents Communication On & Four Agents Communication Off & Four Agents Communication On \\
1.754699432                  & 1.891046696                 & 1.70173354                     & 1.648813013                   & 1.601842272                   & 1.607461362                  \\
1.848926535                  & 1.819475691                 & 1.925419663                    & 1.780157559                   & 1.779689534                   & 1.895588258                  \\
1.93864839                   & 1.918586433                 & 1.796863861                    & 1.940960001                   & 1.850440235                   & 1.267304721                  \\
1.683400257                  & 1.921301512                 & 1.730690704                    & 1.617868891                   & 1.723356478                   & 1.848903254                  \\
1.888883526                  & 1.776940208                 & 1.885341335                    & 1.739270059                   & 2.123164931                   & 1.634528326
\end{tabular}
\end{table}

\begin{table}[]
\centering
\caption{My caption}
\label{tab:UnknownResults3}
\begin{tabular}{llllll}
Two Agents Communication Off & Two Agents Communication On & Three Agents Communication Off & Three Agents Communication On & Four Agents Communication Off & Four Agents Communication On \\
1.34718793                   & 1.263492761                 & 1.587480048                    & 1.662888015                   & 1.142464161                   & 1.420102124                  \\
1.422180449                  & 1.506149114                 & 1.514389448                    & 1.503513771                   & 1.270101299                   & 1.641719208                  \\
1.219717214                  & 1.290602815                 & 1.585903944                    & 1.508783685                   & 1.575773144                   & 1.755198054                  \\
1.574683191                  & 1.554951286                 & 1.756107065                    & 1.395482148                   & 1.355890636                   & 1.68488027                   \\
1.595299188                  & 1.590142433                 & 1.657783394                    & 1.187818501                   & 1.358847806                   & 1.569896654
\end{tabular}
\end{table}

\begin{table}[]
\centering
\caption{My caption}
\label{tab:UnknownResults4}
\begin{tabular}{lll}
Two Agents   & Three Agents & Four Agents  \\
1.029841529  & 0.6968543883 & 0.5669806945 \\
1.010616991  & 0.924513978  & 0.8383721267 \\
0.8365419023 & 0.8431262423 & 0.6927241998 \\
0.8021691138 & 0.7923846054 & 0.8605066193 \\
0.9296503017 & 0.8173152124 & 0.7269435286
\end{tabular}
\end{table}

\begin{table}[]
\centering
\caption{My caption}
\label{tab:UnknownResults5}
\begin{tabular}{llllll}
Two Agents Communication Off & Two Agents Communication On & Three Agents Communication Off & Three Agents Communication On & Four Agents Communication Off & Four Agents Communication On \\
1.452359363                  & 1.409749167                 & 1.799558444                    & 1.541205166                   & 1.543556313                   & 1.567536056                  \\
1.596379895                  & 1.553312301                 & 1.494943593                    & 1.261160517                   & 1.333360997                   & 1.59790598                   \\
1.300157322                  & 1.174255157                 & 1.394356845                    & 1.833281405                   & 1.495561333                   & 1.414808011                  \\
1.433076281                  & 1.667413132                 & 1.7718827                      & 1.335253798                   & 1.370944507                   & 1.445649311                  \\
1.300275353                  & 1.576482942                 & 1.564199261                    & 1.378793385                   & 1.419922887                   & 1.509276382
\end{tabular}
\end{table}

\begin{table}[]
\centering
\caption{My caption}
\label{tab:UnknownResults6}
\begin{tabular}{llllll}
Two Agents Communication Off & Two Agents Communication On & Three Agents Communication Off & Three Agents Communication On & Four Agents Communication Off & Four Agents Communication On \\
1.634708925                  & 1.6665927                   & 1.742239874                    & 1.601128368                   & 1.624078023                   & 1.615004128                  \\
1.628209521                  & 1.630013957                 & 1.724456453                    & 1.61663653                    & 1.631243796                   & 1.566389705                  \\
1.71569864                   & 1.69431785                  & 1.614446562                    & 1.692943124                   & 1.699282765                   & 1.618818691                  \\
1.675246877                  & 1.648490387                 & 1.61786593                     & 1.683234591                   & 1.597384299                   & 1.691945077                  \\
1.739171532                  & 1.621668697                 & 1.624639295                    & 1.652407035                   & 1.665395842                   & 1.780915051
\end{tabular}
\end{table}
